# Supplementary material for: When Noisy Labels Meet Long Tail Dilemmas: A Representation Calibration Method
Source: arXiv:2211.10955 source file (2023-11-07)
Supplement: Supplementary file 1 [file appendix.tex]

\documentclass[10pt,twocolumn,letterpaper]{article}

\usepackage{iccv}
\usepackage{times}
\usepackage{epsfig}
\usepackage{graphicx}
\usepackage{amsmath}
\usepackage{amssymb}
\usepackage{color}
\usepackage{multicol}
\usepackage{multirow}
\usepackage{makecell}
\usepackage{booktabs}
\usepackage{bbm}
\usepackage{bm} 
\usepackage{enumitem}
\usepackage{algorithm}
\usepackage{algorithmic}
\usepackage{amsthm}
\usepackage{caption}
\usepackage{subcaption}
\usepackage{soul}
\usepackage{enumerate}

\begin{document}

\appendix

\onecolumn
\begin{center}
    \Large\bf Appendix
\end{center}

\input{sections/proof.tex}
\input{sections/complementary_exper.tex}
\input{sections/addition_related.tex}

{\small
\bibliographystyle{ieee_fullname}
\bibliography{egbib}
}

\end{document}
